# Supplementary material for: Robust Intervention in Networks
Source: arXiv:2501.00235 source file (2025-02-27)
Supplement: Supplementary file 1 [file online_appendix.pdf]

# Online Appendix to Robust Intervention in Networks

Daeyoung Jeong Tongseok Lim Euncheol Shin*

February 27, 2025

**Abstract**

We show that Property B holds if and only if $(\psi^0 + \psi) \notin Z$. We also provide additional sufficient conditions under which Property B holds, along with a graphical example of the two-agent case.

## 1 Proof of Equivalence

Property B in the main text requires that the solution to the DM's robust optimization problem contains no zero entries (non-negligence condition).

Recall that the objective function $f : \mathbb{R}^n \times \mathcal{B} \to \mathbb{R}$ is defined as

$$f(\mathbf{x}, \mathbf{B}) = \frac{1}{2}\big(\langle \mathbf{x}, \mathbf{M}\mathbf{x}\rangle + \langle \mathbf{x}, \mathbf{B}\mathbf{x}\rangle + \langle \mathbf{x}, \mathbf{C}\mathbf{x}\rangle - 2\langle \varphi, \mathbf{x}\rangle + \underbrace{||\mathbf{z}||^2 + ||\mathbf{C}^{\frac{1}{2}}\mathbf{x}^0||^2}_{\text{constant}}\big),$$

where $\varphi = \psi^0 + \psi$ with $\psi^0 = \mathbf{C}\mathbf{x}^0$ and $\psi = \sum_{i=1}^n z_i \mathbf{m}_i$. Define $g_i(\mathbf{x}) = \max_{\mathbf{B}_i \in \mathcal{B}_i} \frac{1}{2}\langle \mathbf{x}, \mathbf{B}_i\mathbf{x}\rangle$ for each $i \in N$, which is convex and has its minimum at $\mathbf{0}$. Let $g(\mathbf{x}) = \sum_{i=1}^n g_i(\mathbf{x})$. Let $\mathbf{x}^*$ be defined as

$$\mathbf{x}^* = \arg\min_{\mathbf{x}\in\mathbb{R}^n} \max_{\mathbf{B}\in\mathcal{B}} f(\mathbf{x}, \mathbf{B}) = \arg\min_{\mathbf{x}\in\mathbb{R}^n} \left[ g(\mathbf{x}) + \frac{1}{2}\langle \mathbf{x}, \mathbf{D}\mathbf{x}\rangle - \langle \varphi, \mathbf{x}\rangle + \text{constant} \right],$$

where $\mathbf{D} = \mathbf{M} + \mathbf{C}$. $\mathbf{x}^*$ is determined by the first-order condition, $\varphi \in \mathbf{D}\mathbf{x}^* + \partial g(\mathbf{x}^*)$, where $\partial g(\mathbf{x})$ denotes the set of subgradients of $g$ at $\mathbf{x}$, defined by

$$\partial g(\mathbf{x}) = \{\mathbf{u} \in \mathbb{R}^n \mid g(\mathbf{y}) - g(\mathbf{x}) \geq \langle \mathbf{u}, \mathbf{y} - \mathbf{x}\rangle \text{ for all } \mathbf{y} \in \mathbb{R}^n\}.$$

*Daeyoung Jeong: School of Economics, Yonsei University, Seoul, Republic of Korea. Email: daeyoung.jeong@gmail.com; Tongseok Lim: Mitchell E. Daniels, Jr. School of Business, Purdue University, IN, USA. Email: lim336@purdue.edu; Eunchol Shin: KAIST College of Business, Seoul, Republic of Korea. Email: eshin.econ@kaist.ac.kr.

The first order condition implies that $\mathbf{x}^*$ has a zero entry if and only if

$$\varphi \in Z = \{\mathbf{D}\mathbf{x} + \partial g(\mathbf{x}) \,|\, \mathbf{x} \text{ has a zero entry}\}. \tag{1}$$

Consequently, Property B in the main text is equivalent to the condition $\varphi \notin Z$.

## 2 Sufficient Conditions with An Example

Roughly speaking, Property B requires that $Z$ is small in $\mathbb{R}^n$. $Z$ is small if and only if $\max_{i,j} \mathbf{v}_{ij}^2$ is relatively smaller than the eigenvalues of $\mathbf{D} = \mathbf{M} + \mathbf{C}$. To illustrate these points, consider a network of two agents. Then, for each $i$, the subgradient is calculated as

$$\partial g_i(\mathbf{x}) = \begin{cases} \{x_1(\mathbf{v}_{i1}^2, t\mathbf{v}_{i1}\mathbf{v}_{i2})^\mathsf{T} \,|\, t \in [-1,1]\} & \text{if } x_1 \neq 0, x_2 = 0, \\ \{x_2(t\mathbf{v}_{i1}\mathbf{v}_{i2}, \mathbf{v}_{i2}^2)^\mathsf{T} \,|\, t \in [-1,1]\} & \text{if } x_1 = 0, x_2 \neq 0. \end{cases}$$

Figure 1 illustrates $Z$ under the assumption of $\mathbf{M} + \mathbf{C} = k\mathbf{I}$ for some $k > 0$ for simplicity. In the left figure, the set $\{\mathbf{x}$ has a zero entry$\}$ is represented as the union of two colored lines. The blue line represents the set of $\mathbf{x}$ with $x_1 = 0$, and the red line represents the set of $\mathbf{x}$ with $x_2 = 0$. Consider a set-valued function $\mathbf{D} + \partial g : \mathbb{R}^2 \to \mathbb{R}^2$ defined as $(\mathbf{D} + \partial g)(\mathbf{x}) = \mathbf{D}(\mathbf{x}) + \partial g(\mathbf{x})$. In the right figure in Figure 1, the blue region is the image of the blue line $\{\mathbf{x} \in \mathbb{R} \,|\, x_1 = 0\}$, and the red region is the image of the red line $\{\mathbf{x} \in \mathbb{R} \,|\, x_2 = 0\}$. Property B requires that $\varphi$ is not contained in either of the two regions in the right figure. Since $k > 0$, the union of the two regions is not only strictly contained in $\mathbb{R}^2$, but also strictly decreases in size as $k$ increases. The union of the two regions is closed. Moreover, the measure of the union is nonzero. Consequently, Property B does not hold generically, and the interior of the complement of $Z$ is not empty.

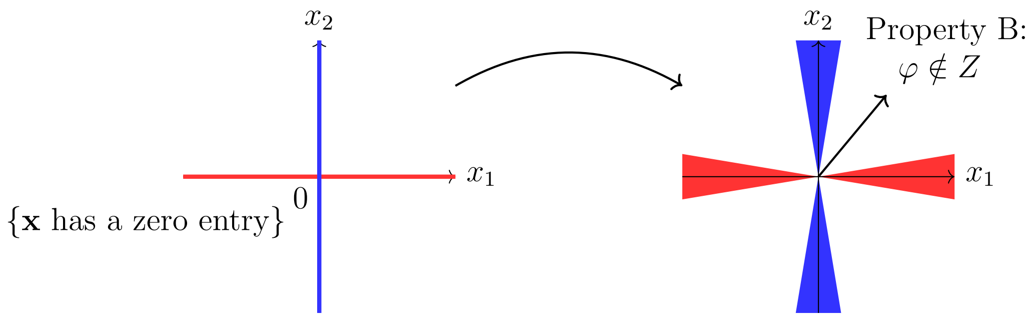


Figure 1: Illustration of $Z$ as an image of $\mathbf{D}\mathbf{x} + \partial g(\mathbf{x})$

We now explain how the size of $Z$ is determined. Without loss of generality, let us consider the size of the red region in the right figure. For a given value of $x_1$ on the horizontal axis in the left figure, the subgradient is a vertical segment in the red region in the right figure. For example, at $\mathbf{x} = (1, 0)$, $\mathbf{D}\mathbf{x} + \partial g(\mathbf{x}) = \{(k + \mathbf{v}_{i1}^2, t\mathbf{v}_{i1}\mathbf{v}_{i2})^\mathsf{T} \mid t \in [-1, 1]\}$. The height of the segment is determined by the values of $\mathbf{v}_{i1}$ and $\mathbf{v}_{i2}$. Thus, when other parameters are equal, Property B holds if the size of the variances becomes sufficiently small. Similarly, for given values of the variance, Property $B$ holds if $k$ is sufficiently large. Furthermore, it follows that for a given $\varepsilon > 0$, there exists $\delta > 0$ such that if $\frac{\max_{i,j} \mathbf{v}_{ij}^2}{\text{smallest eigenvalue of } \mathbf{D}} < \delta$, then there exists a modified target $\widetilde{\mathbf{z}}$ of $\mathbf{z}$ such that $|\widetilde{\mathbf{z}} - \mathbf{z}| < \varepsilon$, and the corresponding optimal intervention $\mathbf{x}^*$ with respect to the new target $\tilde{\mathbf{z}}$ has no zero entry.
